# Supplementary material for: Ionization-induced Long-lasting Orientation of Symmetric-top Molecules
Source: arXiv:2211.08795 ancillary file (2022-11-16)
Supplement: Supplementary file 1 [file Supplemental_Material.pdf]

# Supplemental Material: Ionization-induced Long-lasting Orientation of Symmetric-top Molecules

Long Xu,[1,*] Ilia Tutunnikov,[1,*] Yehiam Prior,[1,†] and Ilya Sh. Averbukh[1,‡]

[1]*AMOS and Department of Chemical and Biological Physics, The Weizmann Institute of Science, Rehovot 7610001, Israel*

Section I summarizes the numerical methods used in classical and quantum simulations of the laser-driven rotational dynamics of symmetric-top molecules. Section II summarizes the molecular properties of methyl fluoride ($CH_3F$) molecule. In Sec. III, we describe the ensemble-averaged long-lasting orientation of symmetric-top molecules in the classical case.

## CONTENTS

I. Numerical Methods: quantum and classical simulations 1
  A. Quantum simulation 1
  B. Classical simulation 2

II. Molecular properties 3

III. The degree of long-lasting orientation (classical formula) 3

References 4

## I. NUMERICAL METHODS: QUANTUM AND CLASSICAL SIMULATIONS

### A. Quantum simulation

The Hamiltonian describing the molecular rotation driven by a two-color laser pulse is given by $H(t) = H_r + H_{\text{int}}$, where $H_r$ is the rotational kinetic energy Hamiltonian and the interaction term is

$$H_{\text{int}} = V_{\text{pol}} + V_{\text{hyp}} + V_{\text{ion}}. \tag{1}$$

The field-polarizability and field-hyperpolarizability interaction terms are given by [1]

$$V_{\text{pol}} = -\frac{1}{2}\sum_{i,j}\alpha_{ij}E_iE_j, V_{\text{hyp}} = -\frac{1}{6}\sum_{i,j,k}\beta_{ijk}E_iE_jE_k. \tag{2}$$

Here $E_i$, $\alpha_{ij}$, and $\beta_{ijk}$ are the components of the field vector, polarizability tensor $\boldsymbol{\alpha}$, and hyperpolarizability tensor $\boldsymbol{\beta}$, respectively. The ionization depletion term $V_{\text{ion}}$ of $CH_3F$ molecules is given by

$$V_{\text{ion}} = -(i/2)\Gamma(\theta,\chi,t), \tag{3}$$

where

$$\Gamma(\theta,\chi,t) = \begin{cases} F(t)|G(\theta,\chi)|^2, & E(t) > 0,\\ F(t)|G(\pi-\theta,\pi+\chi)|^2, & E(t) < 0,\end{cases} \tag{4}$$

the field factor is [2, 3]

$$F(t) = \frac{\kappa}{2}\left(\frac{4\kappa^2}{|E(t)|}\right)^{2/\kappa-1}\exp\left[-\frac{2\kappa^3}{3|E(t)|}\right], \tag{5}$$

---

* These authors contributed equally to this work
† yehiam.prior@weizmann.ac.il
‡ ilya.averbukh@weizmann.ac.il

and $\kappa = \sqrt{2I_p}$ with $I_p$ as the ionization energy. To reproduce the angle dependence of the ionization rate shown in [3], the structure factor is modeled as

$$G(\theta, \chi) = \left[\sin(\theta) + \frac{3}{2}\sin(2\theta)\right] G_1(\chi), \tag{6}$$

where

$$G_1(\chi) = \begin{cases} \sqrt{1+\sin(3\chi)}, & 0 \le \chi < 7\pi/6, \\ -\sqrt{1+\sin(3\chi)}, & 7\pi/6 \le \chi < 11\pi/6, \\ \sqrt{1+\sin(3\chi)}, & 11\pi/6 \le \chi < 2\pi. \end{cases} \tag{7}$$

In the simulations, the wave function $|\Psi(t)\rangle$ is expressed in the basis set of $|JKM\rangle$, where the quantum numbers $J$, $K$, and $M$ correspond to the magnitude of the angular momentum, projection of the angular momentum on the molecular symmetry axis, and projection of angular momentum on the laboratory $Z$ axis. We use the random phase wave functions method (see, e.g. [4]) to simulate the behavior of the thermal ensemble and the initial state is given by

$$|\psi_l\rangle = \sum_{JKM} \sqrt{\frac{\epsilon_K e^{-E_{JK}/(k_B T)}}{\mathcal{Z}}} |JKM\rangle e^{i\varphi_{l,JKM}}, \tag{8}$$

where $\mathcal{Z}$ is the partition sum, $E_{JK}$ is the energy/eigenvalue corresponding to $|JKM\rangle$ state, $k_B$ is the Boltzmann constant, $T$ is the temperature, and $\varphi_{l,JKM} \in [0, 2\pi)$ is a random number. The sum runs over all the thermally populated eigenstates $|JKM\rangle$. For the $CH_3F$ molecule, the statistical weight due to the nuclear spin statistics is given by [5]

$$\epsilon_K = \frac{(2I_{\rm spin}+1)^3}{3}\left[1 + \frac{2\cos(2\pi K/3)}{(2I_{\rm spin}+1)^2}\right], \tag{9}$$

with $I_{\rm spin} = 1/2$. The time-dependent Schrödinger equation $i\hbar\partial_t|\psi_l(t)\rangle = H(t)|\psi_l(t)\rangle$ is solved by numerical exponentiation of the Hamiltonian matrix (see Expokit [6]). As a result, the time-dependent degree of orientation is given by the average

$$\langle\cos(\theta)\rangle(t) = \frac{1}{L}\sum_{l=1}^{L} \langle\cos(\theta)\rangle_l(t), \tag{10}$$

where $L$ is the number of initial states used, $\langle\cos(\theta)\rangle_l(t) \equiv \langle\psi_l(t)|\cos(\theta)|\psi_l(t)\rangle / \langle\psi_l(t)|\psi_l(t)\rangle$ is the orientation factor of surviving neutral molecules, obtained for the $l$-th initial state, $|\psi_l\rangle$.

### B. Classical simulation

We use the Monte Carlo approach to simulate the behavior of a classical ensemble. Initially, $N = 10^7$ sample molecules are isotropically distributed in space. Their angular velocities are given by the Boltzmann distribution $P(\Omega_i) \propto \exp[-I_i\Omega_i^2/(2k_BT)]$, where $i = a, b, c$ refers to the molecular principal axes of inertia. For each sample molecule, the rotational dynamics in the rotating molecular frame is described by Euler's equations [7]

$$\mathbf{I}\dot{\boldsymbol{\Omega}} = (\mathbf{I}\boldsymbol{\Omega}) \times \boldsymbol{\Omega} + \mathbf{T}, \tag{11}$$

where $\mathbf{I} = \mathrm{diag}(I_a, I_b, I_c)$ is the moment of inertia tensor, $\boldsymbol{\Omega} = (\Omega_a, \Omega_b, \Omega_c)$ is the angular velocity, and $\mathbf{T} = (T_a, T_b, T_c)$ is the torque due to the interactions with the two-color laser field. The torque is given by $\mathbf{T} = [\boldsymbol{\alpha}\mathbf{E}_{mol}] \times \mathbf{E}_{mol} + [\mathbf{E}_{mol}\boldsymbol{\beta}\mathbf{E}_{mol}] \times \mathbf{E}_{mol}/2$. Here, $\mathbf{E}_{mol}$ is the representation of the electric field vector in the basis of the molecular principal axes. The relation between the laboratory and the rotating molecular frames is parametrized by a quaternion, $q = (q_0, q_1, q_2, q_3)$ [8, 9]. The quaternion's equation of motion is $\dot{q} = q\Omega/2$, where the quaternions multiplication rule is assumed, and $\Omega = (0, \Omega_a, \Omega_b, \Omega_c)$. A more detailed description of the classical simulations can be found in [10, 11].

As a consequence of ionization depletion, the orientation factor is obtained by averaging over all neutral molecules

$$\langle\cos(\theta)\rangle(t) = \sum_{n=1}^{N} \rho(\theta_n, \chi_n, t)\cos(\theta_n), \tag{12}$$

TABLE I. Molecular constants (in atomic units) for $CH_3F$.

| Parameter | Value | Parameter | Value |
|---|---|---|---|
| $I_a$ | 20982 | $I_b = I_c$ | 129238 |
| $\alpha_{aa}$ | 18.38 | $\alpha_{bb} = \alpha_{cc}$ | 16.76 |
| $\beta_{aaa}$ | −40.449 | $\beta_{abb} = \beta_{acc}$ | −26.970 |
| $\beta_{bbb} = -\beta_{bcc}$ | 11.019 | $I_p$ | 0.461 |

where the relative weight (non-ionized fraction) of the $n$-th molecule is

$$\rho(\theta_n, \chi_n, t) = N_{\text{neu}}^{-1} \exp\left[-\int_0^t \Gamma(\theta_n, \chi_n, t')\, dt'\right]. \tag{13}$$

and the total number of surviving neutral molecules is

$$N_{\text{neu}} = \sum_{n=1}^{N} \exp\left[-\int_0^t \Gamma(\theta_n, \chi_n, t')\, dt'\right], \tag{14}$$

Here, $\theta_n$ and $\chi_n$ are the time-dependent angles of the $n$-th molecule. The population of surviving neutral molecules is defined as $N_{\text{neu}}/N$.

## II. MOLECULAR PROPERTIES

Table I lists the molecular constants of $CH_3F$. Here, $a, b, c$ correspond to the principal molecular axes of inertia. Moments of inertia ($I_{a,b,c}$) and polarizabilities are taken from NIST [density functional theory (DFT), Coulomb-attenuating method with Becke three-parameter Lee-Yang-Parr functional and augmented correlation-consistent polarized valence triple zeta Gaussian basis set (CAM-B3LYP/aug-cc-pVTZ)] [12]. Hyperpolarizabilities are from [13], and the ionization energy, $I_p$ is from [14].

## III. THE DEGREE OF LONG-LASTING ORIENTATION (CLASSICAL FORMULA)

In this Section, we derive an approximate classical formula for the degree of long-lasting orientation [11]. Since the long-lasting orientation manifests itself under field-free conditions, we begin by considering the free motion of a single classical symmetric top. The free motion of the unit vector $\mathbf{a}$, pointing along the rotational symmetry axis of the molecule, is given by a simple vectorial differential equation $\dot{\mathbf{a}} = (\mathbf{L}/I) \times \mathbf{a}$. Here, $\mathbf{L}$ is the conserved angular momentum vector, $I$ is the moment of inertia along the orthogonal axes $b$ and $c$ ($I_a > I_b = I_c \equiv I$ for an oblate top and $I_a < I$ for a prolate top). The solution to this equation is given by

$$\mathbf{a}(t) = \mathbf{L}\frac{\mathbf{L}\cdot\mathbf{a}(0)}{L^2} + \left[\mathbf{a}(0) - \mathbf{L}\frac{\mathbf{L}\cdot\mathbf{a}(0)}{L^2}\right]\cos\left(\frac{L}{I}t\right) + \frac{\mathbf{L}}{L}\times\mathbf{a}(0)\sin\left(\frac{L}{I}t\right), \tag{15}$$

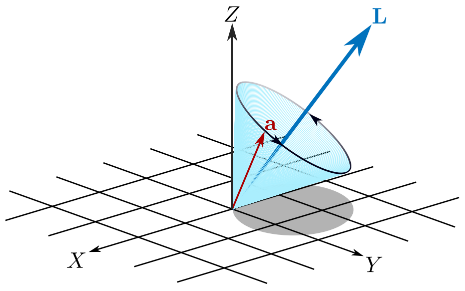


FIG. 1. Illustration of the vector $\mathbf{a}$ precessing about the angular momentum vector $\mathbf{L}$ with a rate of $L/I$, see Eq. (15). The tip of $\mathbf{a}$ describes a circle, while the arrow lies on the surface of a cone. The figure is taken from [11].

where $L$ is the magnitude of angular momentum and $\mathbf{a}(0)$ is vector $\mathbf{a}$ at $t=0$, where $t=0$ defines the end of the two-color pulse (when the free motion begins). The above equation describes precession of $\mathbf{a}$ around $\mathbf{L}$ at a rate $L/I$ (see Fig. 1). In the special case of a linear molecule, $L_a = \mathbf{L}\cdot\mathbf{a}(0) = 0$, so that Eq. (15) reduces to

$$\mathbf{a}(t) = \mathbf{a}(0)\cos\left(\frac{L}{I}t\right) + \frac{\mathbf{L}}{L}\times\mathbf{a}(0)\sin\left(\frac{L}{I}t\right). \tag{16}$$

Equation (16) describes a uniform rotation of $\mathbf{a}$ in a plane perpendicular to the angular momentum vector $\mathbf{L}$.

The degree of long-lasting orientation can be obtained by considering the ensemble average projection of the molecular axis $\mathbf{a}$ on the laboratory $Z$ axis, $\cos(\theta) = \mathbf{e}_Z\cdot\mathbf{a}$, and then evaluating its time average

$$\overline{\langle\cos(\theta)\rangle} = \lim_{\tau\to\infty}\frac{1}{\tau}\int_0^{\tau}\langle\mathbf{e}_Z\cdot\mathbf{a}(t)\rangle\,dt. \tag{17}$$

Next, we exchange the order of the ensemble and time averaging. The time average of $\cos(\theta)$ is obtained from Eq. (15) and it reads

$$\overline{\cos(\theta)} = \frac{(L_Z)_f(L_a)_f}{L_f^2}, \tag{18}$$

where $L_Z = \mathbf{e}_Z\cdot\mathbf{L}$, $L_a = \mathbf{a}\cdot\mathbf{L}$, and subindex $f$ denotes that all the quantities are taken after the pulse. Since the field-polarizability interaction potential depends only on the polar angle $\theta$, the canonically conjugate angular momenta $L_Z$ and $L_a$ are conserved [11]. As a consequence, Eq. (18) becomes

$$\overline{\cos(\theta)} = \frac{L_Z L_a}{L_f^2}, \tag{19}$$

where $L_Z$ and $L_a$ are taken before the pulse. At this stage, we can conclude that the long-lasting orientation is strictly zero when the initial temperature is zero and/or in the limit of a linear rotor. In the first case, $L_Z = L_a = 0$, while in the second case $L_a = 0$, because $I_a = 0$ for linear molecules.

---


[1] A. D. Buckingham, Permanent and induced molecular moments and long-range intermolecular forces, in *Advances in Chemical Physics* (John Wiley & Sons, New York, 2007) pp. 107–142.

[2] O. I. Tolstikhin, T. Morishita, and L. B. Madsen, Theory of tunneling ionization of molecules: Weak-field asymptotics including dipole effects, Phys. Rev. A **84**, 053423 (2011).

[3] P. M. Kraus, O. I. Tolstikhin, D. Baykusheva, A. Rupenyan, J. Schneider, C. Z. Bisgaard, T. Morishita, F. Jensen, L. B. Madsen, and H. J. Wörner, Observation of laser-induced electronic structure in oriented polyatomic molecules, Nat. Commun. **6**, 7039 (2015).

[4] S. Kallush and S. Fleischer, Orientation dynamics of asymmetric rotors using random phase wave functions, Phys. Rev. A **91**, 063420 (2015).

[5] R. S. McDowell, Rotational partition functions for symmetric-top molecules, J. Chem. Phys. **93**, 2801 (1990).

[6] R. B. Sidje, Expokit: A software package for computing matrix exponentials, ACM Trans. Math. Softw. **24**, 130 (1998).

[7] H. Goldstein, C. Poole, and J. Safko, *Classical Mechanics* (Addison Wesley, San Francisco, CA, 2002).

[8] J. B. Kuipers, *Quaternions and Rotation Sequences: A Primer with Applications to Orbits, Aerospace and Virtual Reality* (Princeton University Press, Princeton, N.J., 1999).

[9] E. A. Coutsias and L. Romero, The quaternions with an application to rigid body dynamics, Sandia Technical Report, SAND2004-0153 (2004).

[10] I. Tutunnikov, J. Floß, E. Gershnabel, P. Brumer, and I. Sh. Averbukh, Laser-induced persistent orientation of chiral molecules, Phys. Rev. A **100**, 043406 (2019).

[11] L. Xu, I. Tutunnikov, Y. Prior, and I. Sh. Averbukh, Long-lasting orientation of symmetric-top molecules excited by two-color femtosecond pulses, Front. Phys. **9**, 689635 (2021).

[12] R. D. Johnson, *NIST Computational chemistry comparison and benchmark database, Release 20*, Tech. Rep. (2019).

[13] D. P. Chong, Theoretical calculations of dipole moments, polarizabilities, and hyperpolarizabilities of HF, OCS, $O_3$, $CH_3F$, and $CH_3Cl$ by local density approximation, J. Chin. Chem. Soc. **39**, 375 (1992).

[14] G. Bieri, L. Åsbrink, and W. Von Niessen, 30.4-nm He(II) photoelectron spectra of organic molecules: Part IV. fluoro-compounds (C, H, F), J. Electron Spectrosc. Relat. Phenom. **23**, 281 (1981).
